# Supplementary material for: Tensor-based Collaborative Filtering With Smooth Ratings Scale
Source: arXiv:2205.05070 source file (2022-05-10)
Supplement: Supplementary file 1 [file appendicies.tex]

\section{Appendices}
\label{appendix}

Note that $\widehat{U} \in \mathbb{R}^{M\times r_1}$,
$\widehat{V} \in \mathbb{R}^{N\times r_2}$,
$\widehat{W} \in \mathbb{R}^{K\times r_3}$ 
correspond to the auxiliary latent space. The latent representation of users, items and ratings in the original space is then represented as:

\begin{equation}
\label{eq:orig_latent_1}
%\[
 U = M^{-\frac{1}{2}}\widehat{U}, 
  V = N^{-\frac{1}{2}}\widehat{V},
  W = K^{-\frac{1}{2}}\widehat{W}
%\]
\end{equation}

Columns of the matrices in equation \ref{eq:orig_latent_1} satisfy orthogonality property that is $U^TMU=I_{r_1}, V^TNV=I_{r_2}, W^TKW=I_{r_3} $.

Instead of the 3d case of users-items-rating representation let's consider the 2d case. The standard folding-in technique  for finding a warm-start user representation of his preferences $p^T_0$ is a solution of the following problem:

$$\|p^T_0 - u^T\Sigma V^T\|^2_2 \to min$$

where $u$ is the user latent representation and matrix $V$ is the latent representation of items.

The solution to this minimization problem is

\begin{equation}
\label{eq:u_solution}
u^T = p^T_0 (V^T)^{-1} \Sigma^{-1}
\end{equation}

Obviously, rating prediction is obtained by

\begin{equation}
\label{eq:r_solution}
r^T = u^T \Sigma V^T
\end{equation}

Substituting $V= \widehat{V} = N^\frac{1}{2}V$ to \ref{eq:u_solution} and \ref{eq:r_solution} and using the properties of orthogonality of matrix V, it may be referred that 

\begin{equation}
u^T = p^T_0 ((N^\frac{1}{2}V)^T)^{-1} = p^T_0(N^{-\frac{1}{2}})^TV^{-T}\Sigma^{-1} = p^T_0(N^{-\frac{1}{2}})^TV\Sigma^{-1}
\end{equation}

\begin{equation}
\label{eq:r_pred}
r^T = p^T_0 (N^{-\frac{1}{2}})^TVV^T(N^{\frac{1}{2}})^T
\end{equation}

From \ref{eq:r_pred} it immediately follows that $r = N^{\frac{1}{2}} VV^T N^{-\frac{1}{2}}p_0$. Aggregating the rating prediction of one user for all users we obtain:

\begin{equation}
\label{eq:r_pred_fin}
r = P_0N^{\frac{1}{2}} VV^T N^{-\frac{1}{2}}
\end{equation}

Finally, changing V by W and N by K in \ref{eq:r_pred_fin}  and incorporating it to  \ref{eq:coffee} instead of $WW^T$ (since we are interested in incorporation of similarity just among users leaving $VV^T$ part unchanged) the final formula for prediction is obtained:

\begin{equation}
R_i \approx VV^TP_iK^{\frac{1}{2}}WW^TK^{-\frac{1}{2}}
\end{equation}
